# Supplementary material for: Evaluation of Causal Structure Learning Algorithms via Risk Estimation
Source: arXiv:2006.15387 source file (2020-06-27)
Supplement: Supplementary file 1 [file Supplement.pdf]

# Supplementary material to "Evaluation of Causal Structure Learning Algorithms via Risk Estimation"

## 1 PROOF OF THEOREM 3.3 OF THE MAIN PAPER

*Proof.* We first consider the case $|\boldsymbol{\iota}| = p$. Then

$$
\begin{aligned}
&\mathbb{E}_{\mathbf{X}_{\bar{\iota}} \sim G^{\star}_{\Theta}} \left[ \hat{R}^{J}_{\bar{\iota},w}(\hat{H}_1, \mathbf{X}_{\bar{\iota}}) - \hat{R}^{J}_{\bar{\iota},w}(\hat{H}_2, \mathbf{X}_{\bar{\iota}}) \right] \\
&\quad = \mathbb{E}_{\mathbf{X}_{\bar{\iota}} \sim G^{\star}_{\Theta}} \left[ \hat{R}^{J}_{\bar{\iota},\text{naive}}(\hat{H}_1, \mathbf{X}_{\bar{\iota}}) - \hat{R}^{J}_{\bar{\iota},\text{naive}}(\hat{H}_2, \mathbf{X}_{\bar{\iota}}) \right] \\
&\quad = \mathbb{E}_{\mathbf{X}_{\bar{\iota}} \sim G^{\star}_{\Theta}} \left[ \frac{1}{p} \sum_{i=1}^{p} \Big( J(\widehat{\mathrm{De}}(\mathbf{X}_{\bar{\iota}}, i), \mathrm{De}(\hat{H}_1(\mathbf{X}_{\bar{\iota}}), i)) - J(\widehat{\mathrm{De}}(\mathbf{X}_{\bar{\iota}}, i), \mathrm{De}(\hat{H}_2(\mathbf{X}_{\bar{\iota}}), i)) \Big) \right. \\
&\quad \overset{\text{A(1)}}{=} \mathbb{E}_{\mathbf{X}_{\bar{\iota}} \sim G^{\star}_{\Theta}} \left[ \frac{1}{p} \sum_{i=1}^{p} \Big( J(\mathrm{De}(G^{\star}, i), \mathrm{De}(\hat{H}_1(\mathbf{X}_{\bar{\iota}}), i)) - J(\mathrm{De}(G^{\star}, i), \mathrm{De}(\hat{H}_2(\mathbf{X}_{\bar{\iota}}), i)) \Big) \right. \\
&\quad = R^{J}_{\boldsymbol{\iota}}(\hat{H}_1) - R^{J}_{\boldsymbol{\iota}}(\hat{H}_2),
\end{aligned}
$$

where A(1) refers to Assumption 1 in the main paper. Hence, in this case $\mathbb{E}_{\mathbf{X}_{\bar{\iota}} \sim G^{\star}_{\Theta}} \left[ \hat{R}^{J}_{\bar{\iota},w}(\hat{H}_1, \mathbf{X}_{\bar{\iota}}) - \hat{R}^{J}_{\bar{\iota},w}(\hat{H}_2, \mathbf{X}_{\bar{\iota}}) \right] = R^{J}_{\boldsymbol{\iota}}(\hat{H}_1) - R^{J}_{\boldsymbol{\iota}}(\hat{H}_2)$, which of course implies that the signs of the left- and right-hand sides must match.

Next, we consider the case $|\boldsymbol{\iota}| < p$. Without loss of generality let us suppose that $R^{J}_{\boldsymbol{\iota}}(\hat{H}_1) > R^{J}_{\boldsymbol{\iota}}(\hat{H}_2)$, so that $\delta = R^{J}_{\boldsymbol{\iota}}(\hat{H}_1) - R^{J}_{\boldsymbol{\iota}}(\hat{H}_2)$. We then have

$$
\begin{aligned}
&\mathbb{E}_{\mathbf{X}_{\bar{\iota}} \sim G^{\star}_{\Theta}} \left[ \hat{R}^{J}_{\bar{\iota},w}(\hat{H}_1, \mathbf{X}_{\bar{\iota}}) - \hat{R}^{J}_{\bar{\iota},w}(\hat{H}_2, \mathbf{X}_{\bar{\iota}}) \right] \\
&\quad = \mathbb{E}_{\mathbf{X}_{\bar{\iota}} \sim G^{\star}_{\Theta}} \left[ \tfrac{|\boldsymbol{\iota}|}{p} \hat{R}^{J}_{\bar{\iota},\text{naive}}(\hat{H}_1, \mathbf{X}_{\bar{\iota}}) + \tfrac{p-|\boldsymbol{\iota}|}{p} \hat{R}^{J}_{\bar{\iota},CV}(\hat{H}_1, \mathbf{X}_{\bar{\iota}}) - \tfrac{|\boldsymbol{\iota}|}{p} \hat{R}^{J}_{\bar{\iota},\text{naive}}(\hat{H}_2, \mathbf{X}_{\bar{\iota}}) - \tfrac{p-|\boldsymbol{\iota}|}{p} \hat{R}^{J}_{\bar{\iota},CV}(\hat{H}_2, \mathbf{X}_{\bar{\iota}}) \right] \\
&\quad = \mathbb{E}_{\mathbf{X}_{\bar{\iota}} \sim G^{\star}_{\Theta}} \left[ \frac{|\boldsymbol{\iota}|}{p} \frac{1}{|\boldsymbol{\iota}|} \sum_{i \in \boldsymbol{\iota}} \Big( J(\widehat{\mathrm{De}}(\mathbf{X}_{\bar{\iota}}, i), \mathrm{De}(\hat{H}_1(\mathbf{X}_{\bar{\iota}}), i)) - J(\widehat{\mathrm{De}}(\mathbf{X}_{\bar{\iota}}, i), \mathrm{De}(\hat{H}_2(\mathbf{X}_{\bar{\iota}}), i)) \Big) \right. \\
&\qquad\qquad \left. + \frac{p - |\boldsymbol{\iota}|}{p} \Big( \hat{R}^{J}_{\bar{\iota},CV}(\hat{H}_1, \mathbf{X}_{\bar{\iota}}) - \hat{R}^{J}_{\bar{\iota},CV}(\hat{H}_2, \mathbf{X}_{\bar{\iota}}) \Big) \right] \\
&\quad \overset{\text{A(1)}}{=} \mathbb{E}_{\mathbf{X}_{\bar{\iota}} \sim G^{\star}_{\Theta}} \left[ \frac{1}{p} \sum_{i \in \boldsymbol{\iota}} \Big( J(\mathrm{De}(G^{\star}, i), \mathrm{De}(\hat{H}_1(\mathbf{X}_{\bar{\iota}}), i)) - J(\mathrm{De}(G^{\star}, i), \mathrm{De}(\hat{H}_2(\mathbf{X}_{\bar{\iota}}), i)) \Big) \right. \\
&\qquad\qquad \left. + \frac{p - |\boldsymbol{\iota}|}{p} \Big( \hat{R}^{J}_{\bar{\iota},CV}(\hat{H}_1, \mathbf{X}_{\bar{\iota}}) - \hat{R}^{J}_{\bar{\iota},CV}(\hat{H}_2, \mathbf{X}_{\bar{\iota}}) \Big) \right]
\end{aligned}
$$

$$
\begin{aligned}
&= \mathbb{E}_{\mathbf{X}_{\bar{\iota}} \sim G^\star_\Theta} \Bigg[ \frac{1}{p} \sum_{i=1}^{p} \Big( J(\mathrm{De}(G^\star, i), \mathrm{De}(\hat{H}_1(\mathbf{X}_{\bar{\iota}}), i)) - J(\mathrm{De}(G^\star, i), \mathrm{De}(\hat{H}_2(\mathbf{X}_{\bar{\iota}}), i)) \Big) \\
&\qquad - \frac{1}{p} \sum_{i \notin \iota} \Big( J(\mathrm{De}(G^\star, i), \mathrm{De}(\hat{H}_1(\mathbf{X}_{\bar{\iota}}), i)) - J(\mathrm{De}(G^\star, i), \mathrm{De}(\hat{H}_2(\mathbf{X}_{\bar{\iota}}), i)) \Big) \\
&\qquad + \frac{p - |\iota|}{p} \Big( \hat{R}^J_{\iota, CV}(\hat{H}_1, \mathbf{X}_{\bar{\iota}}) - \hat{R}^J_{\iota, CV}(\hat{H}_2, \mathbf{X}_{\bar{\iota}}) \Big) \Bigg] \\
&= R^J_{\iota}(\hat{H}_1) - R^J_{\iota}(\hat{H}_2) \\
&\quad - \mathbb{E}_{\mathbf{X}_{\bar{\iota}} \sim G^\star_\Theta} \Bigg[ \frac{1}{p} \sum_{i \notin \iota} \Big( J(\mathrm{De}(G^\star, i), \mathrm{De}(\hat{H}_1(\mathbf{X}_{\bar{\iota}}), i)) - J(\mathrm{De}(G^\star, i), \mathrm{De}(\hat{H}_2(\mathbf{X}_{\bar{\iota}}), i)) \Big) \\
&\qquad - \frac{p - |\iota|}{p} \Big( \hat{R}^J_{\iota, CV}(\hat{H}_1, \mathbf{X}_{\bar{\iota}}) - \hat{R}^J_{\iota, CV}(\hat{H}_2, \mathbf{X}_{\bar{\iota}}) \Big) \Bigg] \\
&= R^J_{\iota}(\hat{H}_1) - R^J_{\iota}(\hat{H}_2) \\
&\quad - \frac{p - |\iota|}{p} \mathbb{E}_{\mathbf{X}_{\bar{\iota}} \sim G^\star_\Theta} \Bigg[ \frac{1}{p - |\iota|} \sum_{i \notin \iota} \Big( J(\mathrm{De}(G^\star, i), \mathrm{De}(\hat{H}_1(\mathbf{X}_{\bar{\iota}}), i)) - J(\mathrm{De}(G^\star, i), \mathrm{De}(\hat{H}_2(\mathbf{X}_{\bar{\iota}}), i)) \Big) \\
&\qquad - \Big( \hat{R}^J_{\iota, CV}(\hat{H}_1, \mathbf{X}_{\bar{\iota}}) - \hat{R}^J_{\iota, CV}(\hat{H}_2, \mathbf{X}_{\bar{\iota}}) \Big) \Bigg] \\
&\overset{\text{A(2)}}{>} R^J_{\iota}(\hat{H}_1) - R^J_{\iota}(\hat{H}_2) - \delta = 0,
\end{aligned}
$$

where A(1) and A(2) refer to Assumptions 1 and 2 in the main paper.

Hence, the sign of $\mathbb{E}_{\mathbf{X}_{\bar{\iota}} \sim G^\star_\Theta} \Big[ \hat{R}^J_{\iota, w}(\hat{H}_1, \mathbf{X}_{\bar{\iota}}) - \hat{R}^J_{\iota, w}(\hat{H}_2, \mathbf{X}_{\bar{\iota}}) \Big]$ is the same as the sign of $R^J_{\iota}(\hat{H}_1) - R^J_{\iota}(\hat{H}_2)$.

□

# 2 ADDITIONAL DETAILS ON THE SIMULATION SET-UP

*R-version and code.* For our simulations we used `R` version 3.6.1. The code of the simulation, together with the list of the used packages and their versions, is available on GitHub at the following link: “https://github.com/marcoeigenmann/Evaluation-of-Causal-Algorithms-via-Risk-Estimation”.

*Signal to noise ratio and scaling.* In the model we used for our simulation study, we can quantify for each node the signal coming from its parents by the variance of this part. Similarly, we can quantify the noise by the variance of its additive noise term. In order to achieve that all variables $X_i$, $i \in [p]$, have unit variance and a signal to noise ratio of 5 for non-source nodes, we did the following. We generated the noise terms according to the distributions described in the main paper. For non-source nodes, we scaled them to have a variance of $1/6$. The signal coming from the parents was then scaled to have variance $5/6$, to obtain a signal-to-noise ratio of 5. The latter was achieved as follows. We started by sampling all non-zero edge weights independently and uniformly from the interval $[-3, -1] \cup [1, 3]$. Next, following a causal order of the nodes, we computed the empirical variance of the sum of all incoming nodes (the signal) for each node. We used this value to compute a scaling factor which was applied to all edge weights of the incoming nodes, to obtain a signal strength of $5/6$. For further details we refer to (Heinze-Deml, Maathuis, & Meinshausen, 2018), which we closely followed.

## 2.1 COMPUTATION OF THE CUT-OFF FOR THE ESTIMATION OF THE DESCENDANTS

We now describe the procedure by which cut-offs were computed for the test statistics used in experiments in the main paper. We note that any ranking procedure (this need not even be a formal statistical test) could be used to rank candidate descendants and various ad-hoc cut-offs could be used in practice. The distributional assumptions below are, in that sense, not essential for the use of our method, but provide just one way to set a cut-off under a Normality assumption.

Following the notation of the main paper, we denote by $\mathbf{X}_{\bar{\iota}}$ realizations of Normal random variables coming from a

SEM. For each intervention $i \in \bar{\iota}$, $\mathbf{X}_{\{i\}}$ is a $n_i \times p$ matrix, where the $j$th column corresponds to $n_i$ realizations of $X_j$ under the intervention on node $X_i$. We denote the $j$th column of $\boldsymbol{X}_{\{i\}}$ by $\left(\boldsymbol{X}_{\{i\}}\right)_{\cdot,j}$, and its $k$th entry by $\left(\boldsymbol{X}_{\{i\}}\right)_{k,j}$. Finally, we define $\left(\bar{\boldsymbol{X}}_{\{i\}}\right)_{\cdot,j} = \sum_{k=1}^{n_i} \frac{1}{n_i}(\boldsymbol{X}_{\{i\}})_{k,j}$.

We consider the following t-statistic:

$$T_{i,j}(\mathbf{X}_{\bar{\iota}}) = \sqrt{\frac{n_0 n_i}{(n_0+n_i)s^2}} \left( (\bar{\boldsymbol{X}}_{\{0\}})_{\cdot,j} - (\bar{\boldsymbol{X}}_{\{i\}})_{\cdot,j} \right),$$

where

$$s^2 = \frac{(n_0-1)s_{0,j}^2 + (n_i-1)s_{i,j}^2}{n_0+n_i-2} \qquad \text{and} \qquad s_{i,j}^2 = \frac{\sum_{k=1}^{n_i} \left( \left(\boldsymbol{X}_{\{i\}}\right)_{k,j} - \left(\bar{\boldsymbol{X}}_{\{i\}}\right)_{\cdot,j} \right)^2}{n_i - 1}.$$

Here a large absolute value of the t-statistic $T_{i,j}(\mathbf{X}_{\bar{\iota}})$ indicates that $X_j$ is a descendant of $X_i$.

For a fixed node $X_j$, if $j \notin \boldsymbol{\iota}$, we consider $T_{i,j}(\mathbf{X}_{\bar{\iota}})$ for each $i \in \boldsymbol{\iota} = \{i_1, \ldots, i_{|\boldsymbol{\iota}|}\}$, yielding $r_j = |\boldsymbol{\iota}|$ t-statistics. If $j \in \boldsymbol{\iota}$, we must omit the case where $i = j$, yielding $r_j = |\boldsymbol{\iota}| - 1$ t-statistics. In total we have $|\boldsymbol{\iota}|(p-1)$ t-statistics.

If the underlying true graph is empty, and the sample size of all interventions in $\boldsymbol{\iota}$ is the same, then the joint distribution of all $|\boldsymbol{\iota}|(p-1)$ t-statistics

$$((T_{i,1} : i \in \boldsymbol{\iota}, i \neq 1), (T_{i,2} : i \in \boldsymbol{\iota}, i \neq 2), \ldots, (T_{i,p} : i \in \boldsymbol{\iota}, i \neq p))$$

follows a multivariate t-distribution with $n_0 + n_i - 2$ degrees of freedom, mean 0, and covariance matrix

$$\Sigma = \begin{pmatrix} B_1 & 0 & 0 & 0 \\ 0 & B_2 & 0 & 0 \\ 0 & 0 & \ddots & 0 \\ 0 & 0 & 0 & B_p \end{pmatrix}, \qquad (1)$$

where $\forall j \in [p]$, $B_j$ is a $r_j \times r_j$ matrix with ones on the diagonal and $n_i/(n_0 + n_i)$ everywhere else.

We set the cut-off above which we consider the absolute value of a t-statistics significant for our descendants estimation to be the $1 - \alpha$ equicoordinate quantile of this distribution for $\alpha = 0.05$. In the case of an empty $G^*$ this controls the family wise error rate at level $\alpha$. The quantiles are computed using the `R` package `mvtnorm`.

# 3 ADDITIONAL SIMULATION RESULTS

## 3.1 PLOTS LIKE FIGURE 1 IN THE MAIN PAPER, FOR DIFFERENT COMBINATIONS OF ALGORITHMS

Here we present results using the proposed risk estimator for further combinations of algorithms than those shown in the main paper. Figures 1 to 5 show the following pairs: $\widehat{GES}$ vs $\widehat{GIES}$, $\widehat{GIES}$ vs $\widehat{ACor}$, $\widehat{GIES}$ vs $\widehat{Empty}$, $\widehat{GES}$ vs $\widehat{Empty}$, and $\widehat{ACor}$ vs $\widehat{Empty}$ (see the main paper). These additional results are broadly consistent with the key observations presented in the main paper.

It is interesting to see that the comparison between the two causal structure learning algorithms, $\widehat{GIES}$ and $\widehat{GES}$, in Figure 1 seems to give relatively good results, even when the difference in true risks is small.

The comparison between $\widehat{GIES}$ and $\widehat{Acor}$ in Figure 2 is handled very well by the risk estimator (bottom plot is green), but the oracle difference in risks is rather large here (top plot is purple), indicating that this is in that sense a relatively "easy" case.

The comparison between $\widehat{GIES}$ and $\widehat{Empty}$ and between $\widehat{GES}$ and $\widehat{Empty}$ in Figures 3 and 4 is more challenging for the risk estimator. We see that we need a larger sample size to get the correct sign.

The comparison between $\widehat{ACor}$ and $\widehat{Empty}$ in Figure 5 is interesting. We see how the top plot is very light blue, indicating that the two graph estimates are not far apart in terms of oracle risks. However, these two graph estimators are very different: $\widehat{Empty}$ contains only one edge and $\widehat{Acor}$ has the correct sparsity but too many descendants (since every undirected edge is interpreted as a possibly directed edge in either direction). Still, the risk estimator performs rather well, except for the sigmoidal log-normal case.

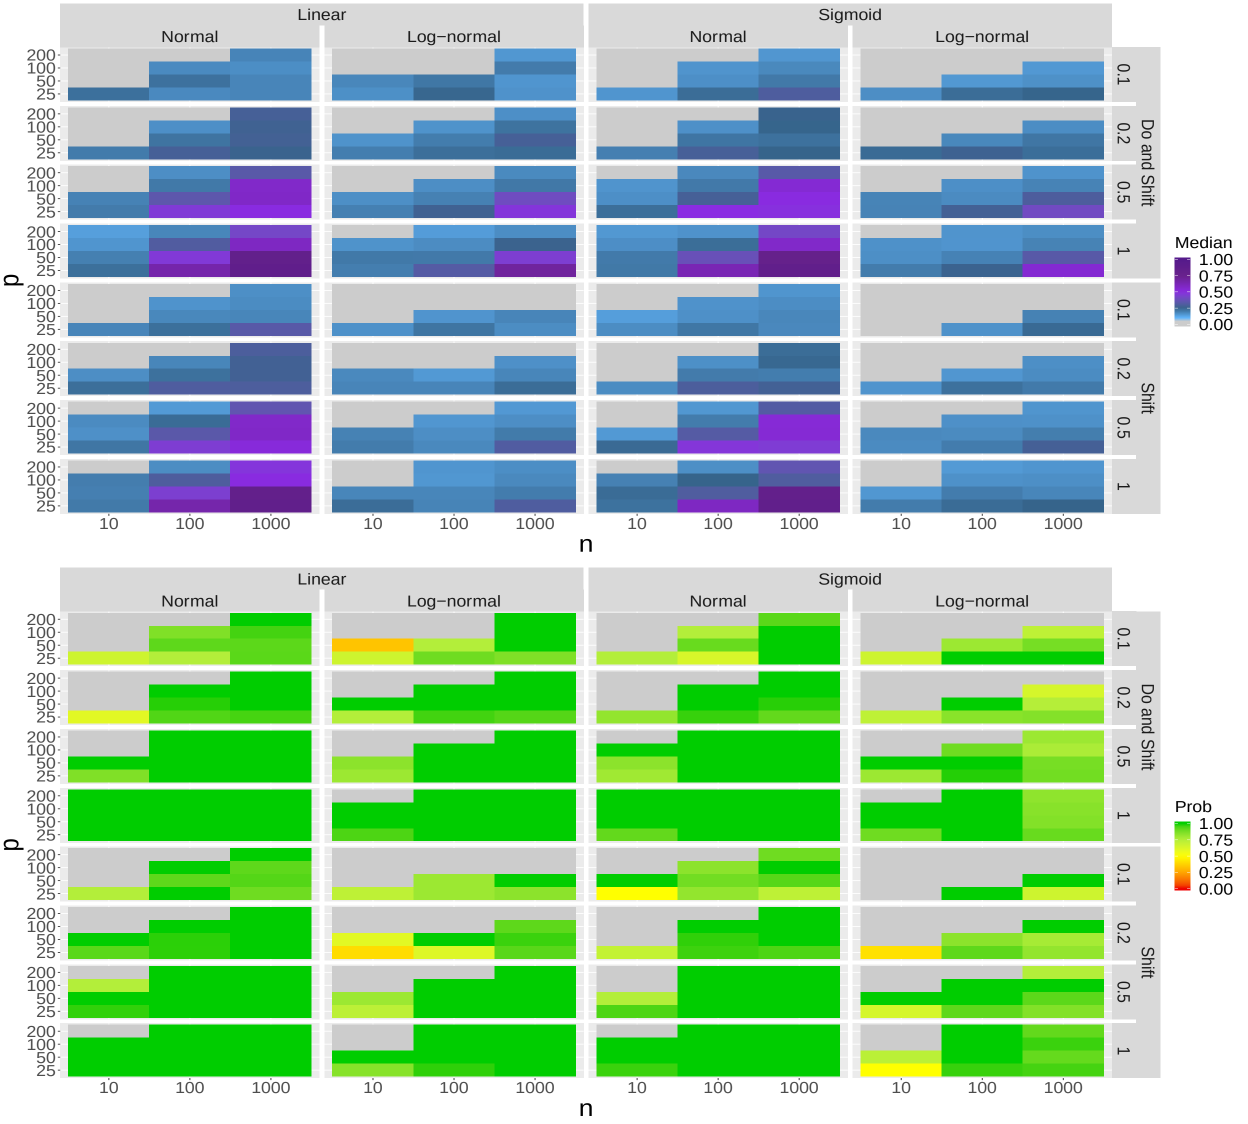


Figure 1: For both the top and bottom panel: Each cell corresponds to a simulation setting, characterized by $p$ (left vertical axis), $n$ (bottom horizontal axis), the link functions and error distribution of them SEM (top horizontal axis) and the type and probability of an intervention (right vertical axis). Top panel: median difference of true risk $R^J_{\imath}(\widehat{GIES}) - R^J_{\imath}(\widehat{GES})$ for different settings. A small value (blue) represents a more difficult situation to evaluate. Bottom panel: empirical probabilities for how often the difference in estimated risk $\widehat{R}^J_{\imath,w}(\widehat{GIES},\cdot) - \widehat{R}^J_{\imath,w}(\widehat{GES},\cdot)$ agrees in sign with the difference of true risk for different settings. A large value (green) means that the risk estimator performed well. In each cell we consider only settings for which the true risks differ by at least $0.1$. A cell is left gray if less than 3 settings are available.

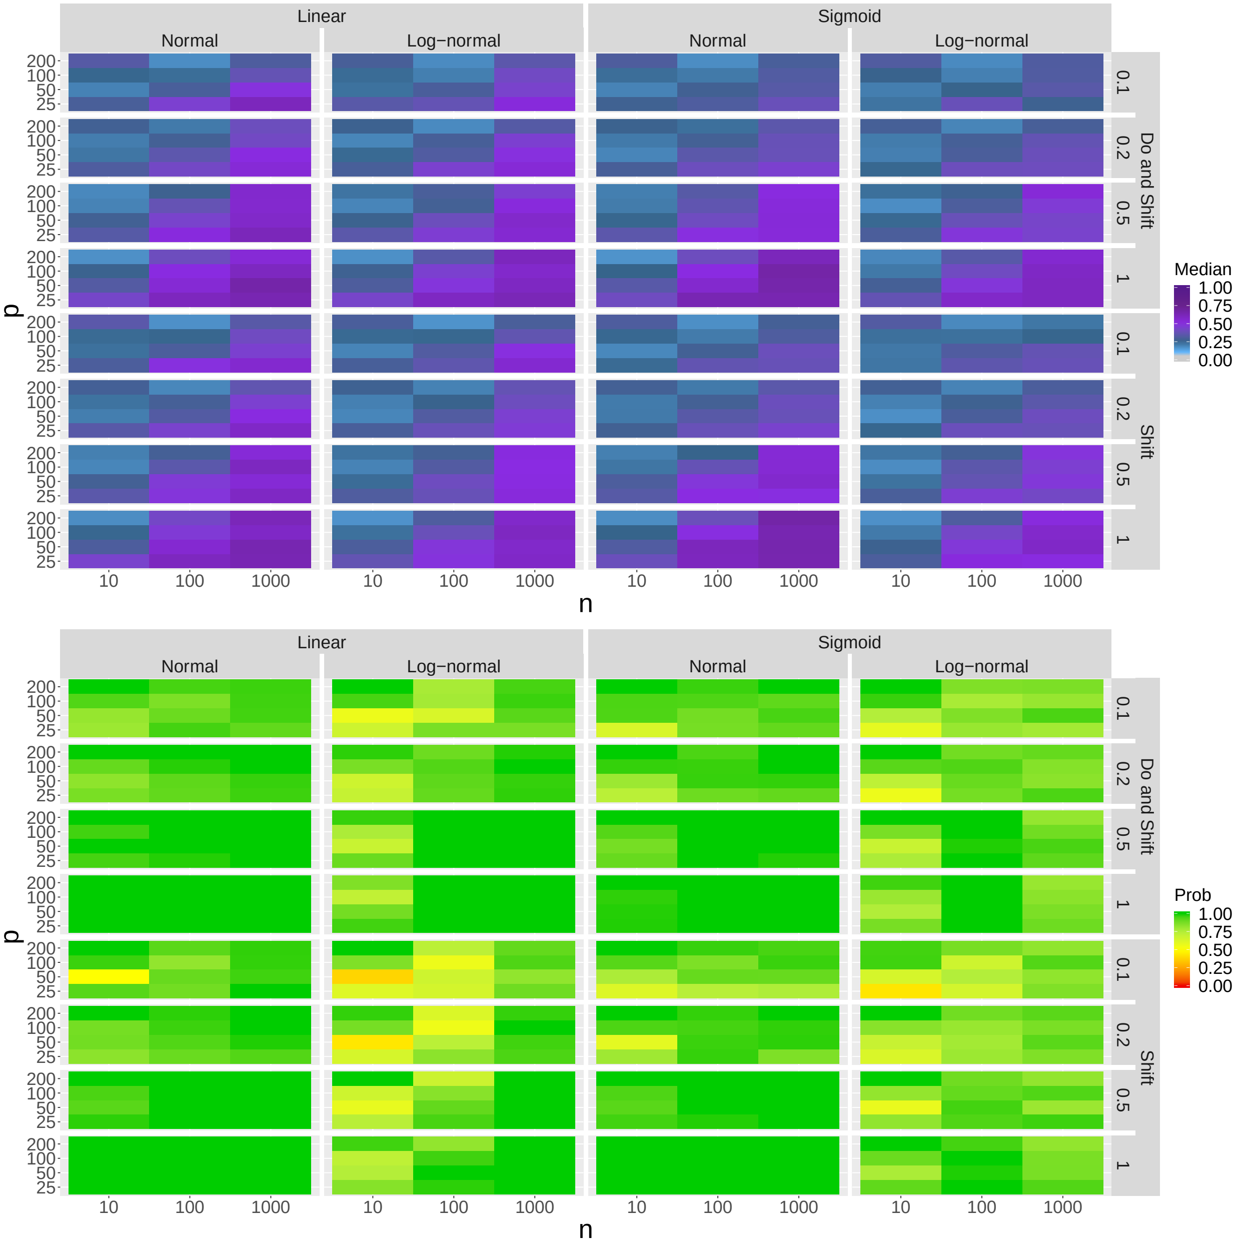


Figure 2: For both the top and bottom panel: Each cell corresponds to a simulation setting, as in Figure 1. Top panel: median difference of true risk $R^J_{\boldsymbol{\iota}}(\widehat{GIES}) - R^J_{\boldsymbol{\iota}}(\widehat{ACor})$ for different settings. A small value (blue) represents a more difficult situation to evaluate. Bottom panel: empirical probabilities for how often the difference in estimated risk $\widehat{R}^J_{\boldsymbol{\iota},w}(\widehat{GIES}, \cdot) - \widehat{R}^J_{\boldsymbol{\iota},w}(\widehat{ACor}, \cdot)$ agrees in sign with the difference of true risk for different settings. A large value (green) means that the risk estimator performed well. In each cell we consider only settings for which the true risks differ by at least $0.1$. A cell is left gray if less than 3 settings are available.

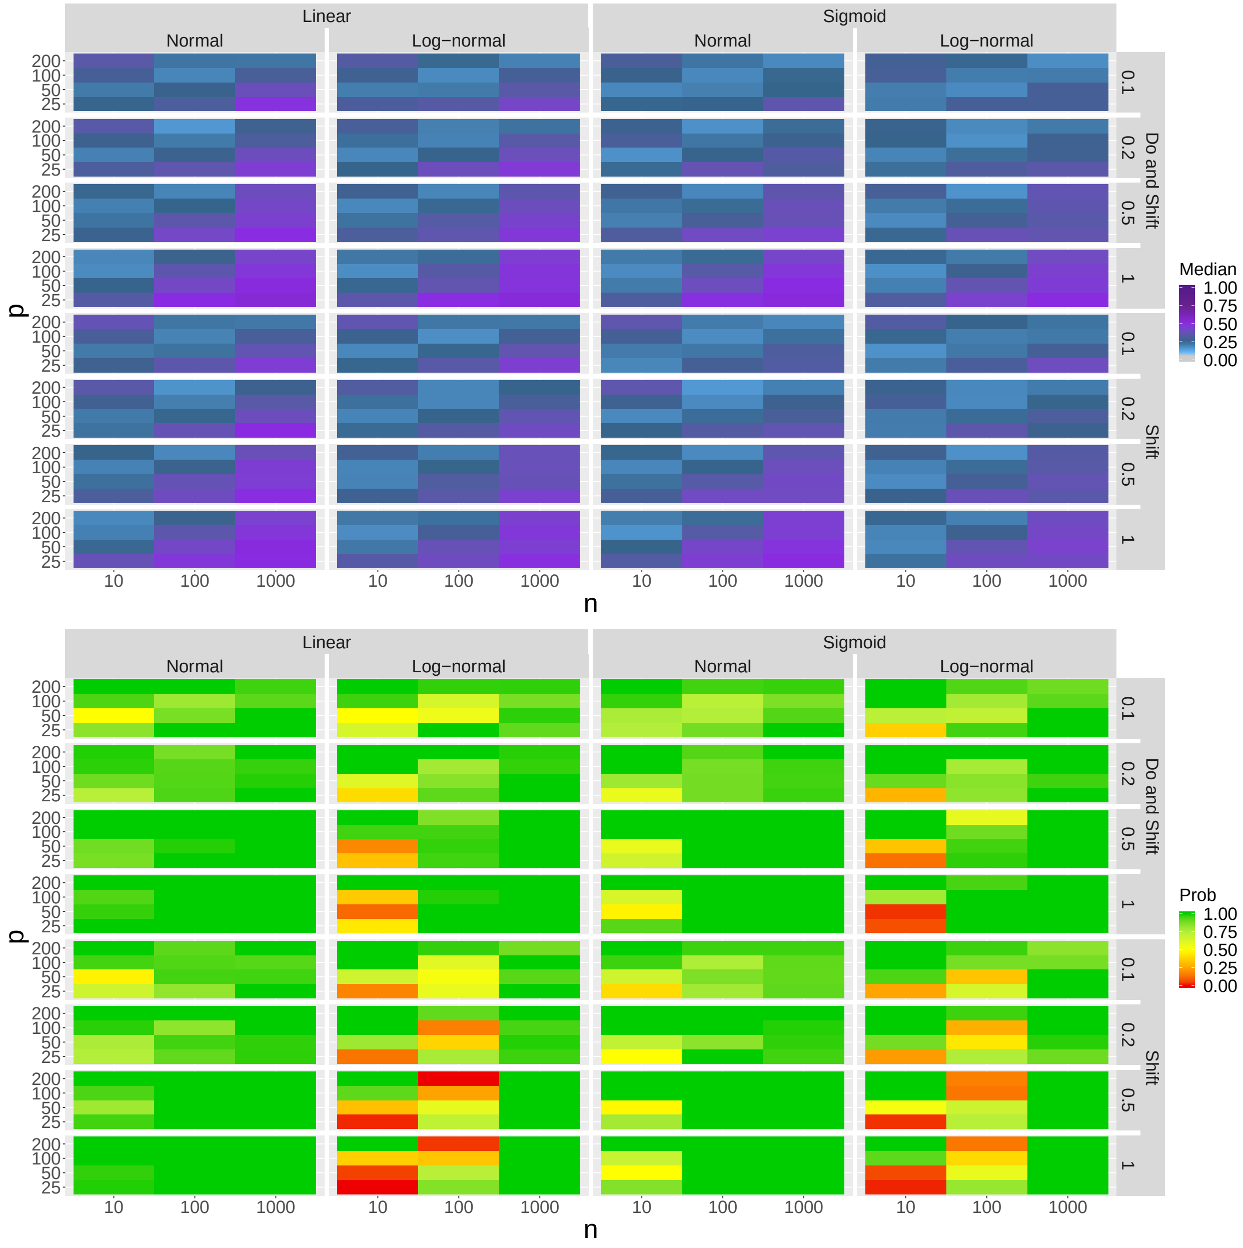


Figure 3: For both the top and bottom panel: Each cell corresponds to a simulation setting, as in Figure 1. Top panel: median difference of true risk $R^J_{\bar{\iota}}(\widehat{GIES}) - R^J_{\bar{\iota}}(\widehat{Empty})$ for different settings. A small value (blue) represents a more difficult situation to evaluate. Bottom panel: empirical probabilities for how often the difference in estimated risk $\widehat{R}^J_{\bar{\iota},w}(\widehat{GIES}, \cdot) - \widehat{R}^J_{\bar{\iota},w}(\widehat{Empty}, \cdot)$ agrees in sign with the difference of true risk for different settings. A large value (green) means that the risk estimator performed well. In each cell we consider only settings for which the true risks differ by at least $0.1$. A cell is left gray if less than $3$ settings are available.

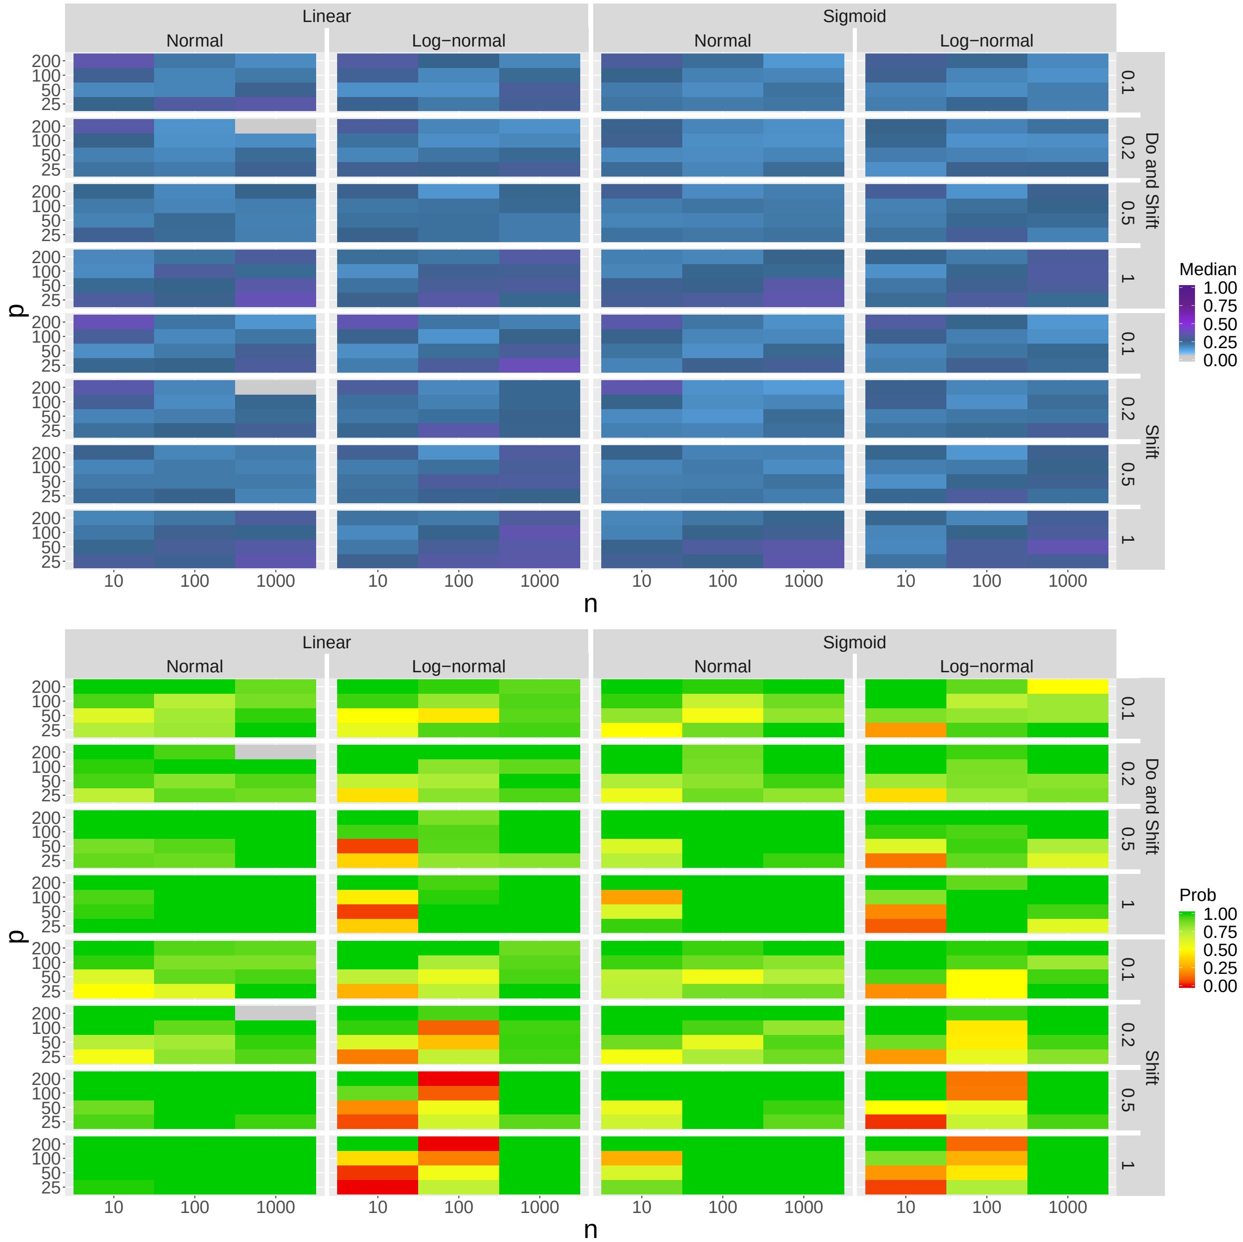


Figure 4: For both the top and bottom panel: Each cell corresponds to a simulation setting, as in Figure 1. Top panel: median difference of true risk $R^J_{\bar{\boldsymbol{\iota}}}(\widehat{GES}) - R^J_{\bar{\boldsymbol{\iota}}}(\widehat{Empty})$ for different settings. A small value (blue) represents a more difficult situation to evaluate. Bottom panel: empirical probabilities for how often the difference in estimated risk $\widehat{R}^J_{\bar{\boldsymbol{\iota}},w}(\widehat{GES},\cdot) - \widehat{R}^J_{\bar{\boldsymbol{\iota}},w}(\widehat{Empty},\cdot)$ agrees in sign with the difference of true risk for different settings. A large value (green) means that the risk estimator performed well. In each cell we consider only settings for which the true risks differ by at least $0.1$. A cell is left gray if less than 3 settings are available.

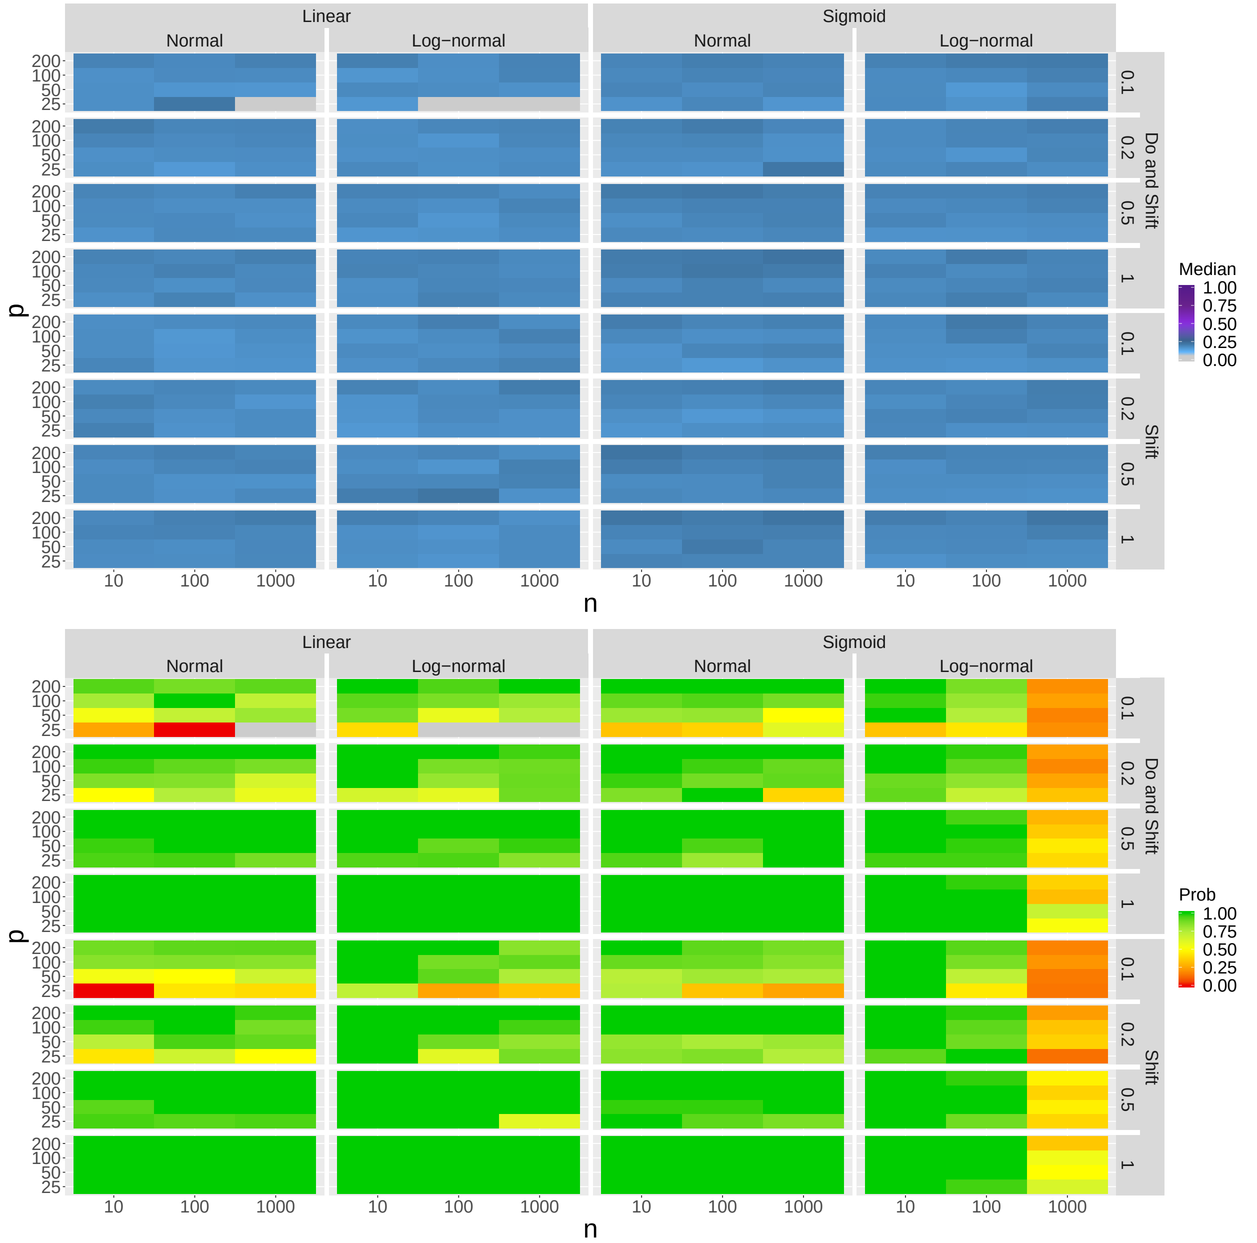


Figure 5: For both the top and bottom panel: Each cell corresponds to a simulation setting, as in Figure 1. Top panel: median difference of true risk $R^J_{\bar{\boldsymbol{\iota}}}(\widehat{Empty}) - R^J_{\bar{\boldsymbol{\iota}}}(\widehat{ACor})$ for different settings. A small value (blue) represents a more difficult situation to evaluate. Bottom panel: empirical probabilities for how often the difference in estimated risk $\widehat{R}^J_{\bar{\boldsymbol{\iota}},w}(\widehat{Empty},\cdot) - \widehat{R}^J_{\bar{\boldsymbol{\iota}},w}(\widehat{ACor},\cdot)$ agrees in sign with the difference of true risk for different settings. A large value (green) means that the risk estimator performed well. In each cell we consider only settings for which the true risks differ by at least $0.1$. A cell is left gray if less than 3 settings are available.

### 3.2 DIRECT EVALUATION OF THE RISK

Often, interest focuses not only on relative performance but on absolute performance, i.e. to ask whether the best performing algorithm is effective in absolute terms or whether perhaps all considered algorithms are performing well or badly.

In Figure 6 we plotted $R^J_{\bar{\imath}}(\widehat{ACor}(\mathbf{X}_{\bar{\imath}}))$ against $\widehat{R}_{\bar{\imath},w}(\widehat{ACor}, \mathbf{X}_{\bar{\imath}})$ for the linear Normal case considering a large sample size, $n = 1000$. In this plot we would like to have points near the diagonal which would indicate an ideal performance of the risk estimator in the sense above. Even though many estimates are good even in the presence of few interventions only, some deviate considerably from the diagonal. In general we observe a larger variability in the result unless we have many interventions, hence we cover a rather larger portion of the nodes.

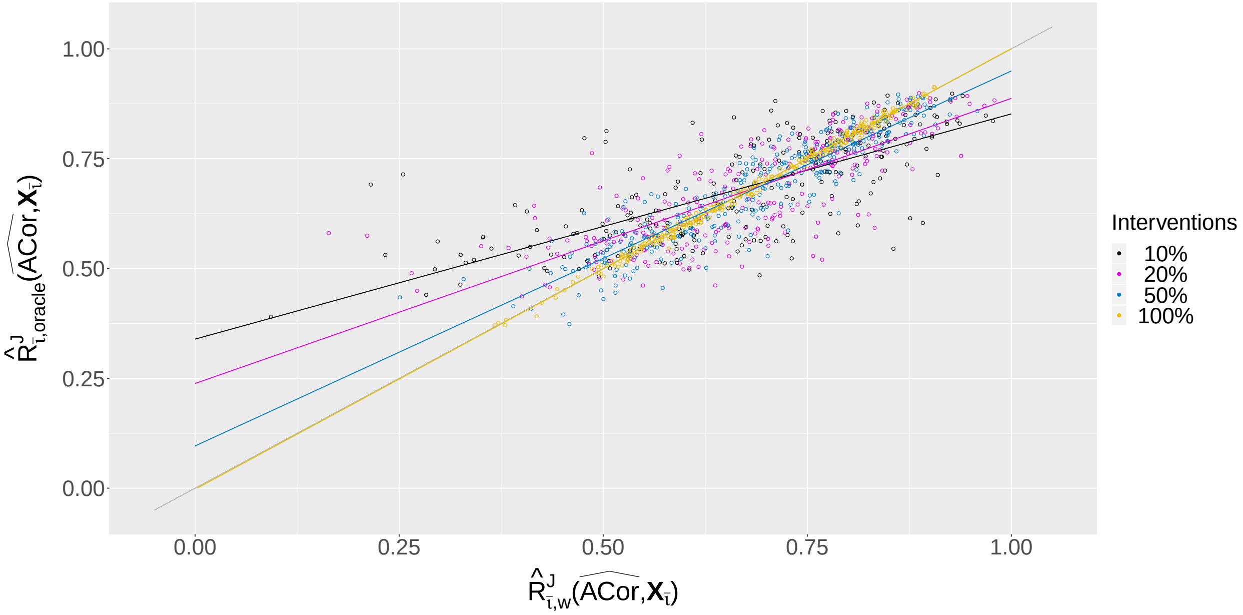


Figure 6: Scatterplot of $\hat{R}^J_{\bar{\imath},oracle}(\widehat{ACor}, \cdot)$ against $\widehat{R}^J_{\bar{\imath},w}(\widehat{ACor}, \cdot)$ with fitted regression lines. The simulation settings consist of: a sample size of 1000, all graph sizes, linear link functions, Normal noise, Do-and-Shift interventions, and different probabilities of an intervention (color-coded). Points on the diagonal indicate a good performance of $\widehat{R}^J_{\bar{\imath},w}(\widehat{ACor}, \cdot)$ when estimating $\widehat{R}^J_{\bar{\imath},oracle}(\widehat{ACor}, \cdot)$.

The bottom line of such scatterplots is common to all algorithms we looked at: for reliable results one needs more interventions than we saw are needed for a proper ranking of the algorithms. At $20\%$ of interventions Kendal correlation values vary between $0.5$ and $0.8$ and with $50\%$ of interventions the values lie above $0.8$ and sometimes also above $0.9$.

One of the possible explanation for this large variability in the presence of few intervened nodes only could be the lack of characterization of the graph through these nodes. The behaviour can be seen in Figures 7 and 8. Both figures consider $\widehat{GES}$, in the former the sample size is $1000$ and in the latter it is $10$. Since we are considering the linear Normal case the descendants selection performs well also for the smaller sample size, see Figure 9. It is visible how points with a value closer to $0.5$ with respect to $R^J_{\bar{\imath}}(\widehat{GES}(\mathbf{X}_{\bar{\imath}}))$ have a larger spread with respect to $\widehat{R}_{\bar{\imath},w}(\widehat{GES}, \mathbf{X}_{\bar{\imath}})$.This basically says that we can have upper bounds for very good results and lower bounds for very bad results.

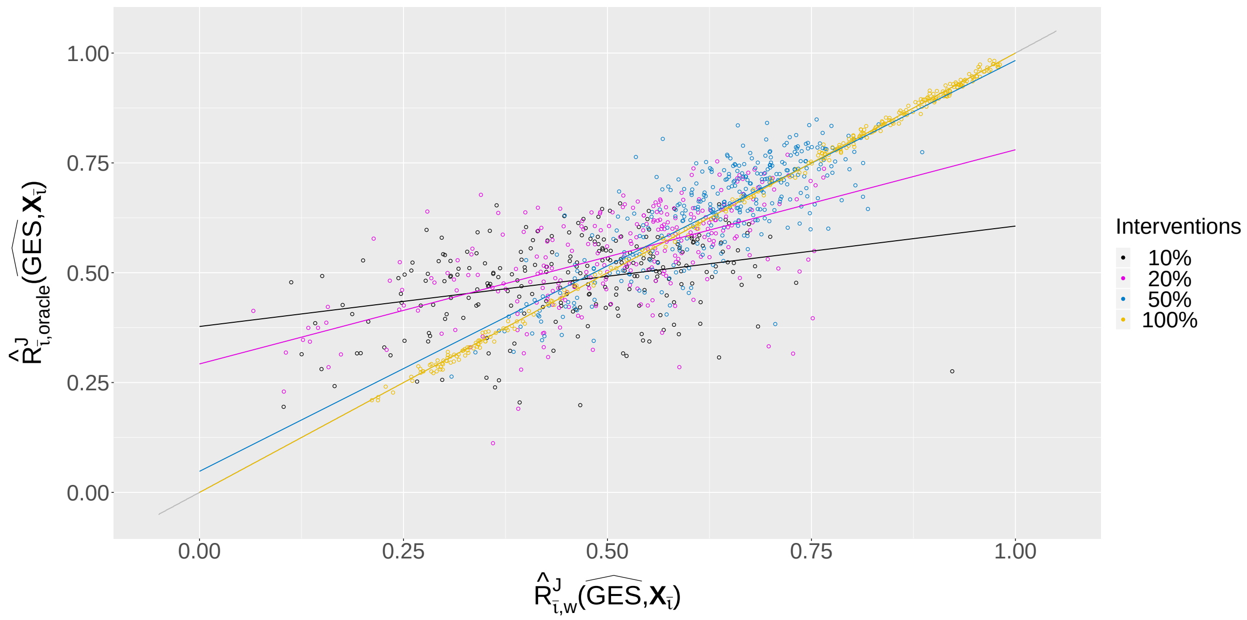


Figure 7: Scatterplot of $\hat{R}^J_{\bar{\iota},oracle}(\widehat{GES},\cdot)$ against $\hat{R}^J_{\bar{\iota},w}(\widehat{GES},\cdot)$ with fitted regression lines. The simulation settings consist of: a sample size of 1000, all graph sizes, linear link functions, Normal noise, Do-and-Shift interventions, and different probabilities of an intervention (color-coded). Points on the diagonal indicate a good performance of $\widehat{R}^J_{\bar{\iota},w}(\widehat{GES},\cdot)$ when estimating $\hat{R}^J_{\bar{\iota}}(\widehat{GES},\cdot)$.

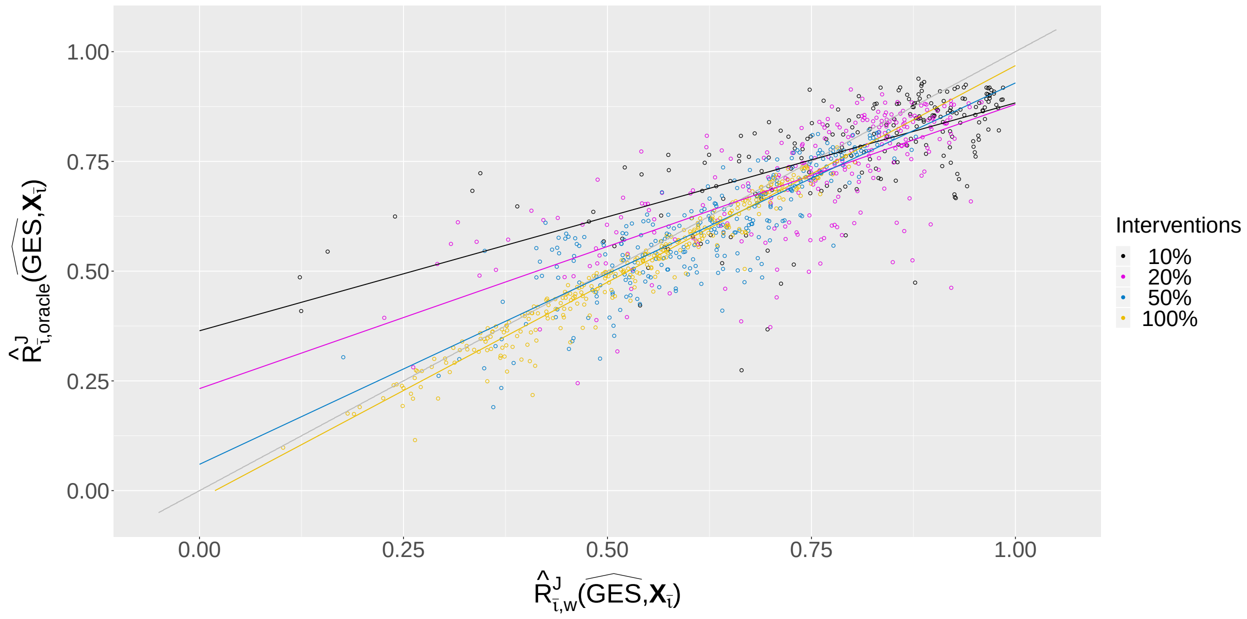


Figure 8: Scatterplot of $\hat{R}^J_{\bar{\iota},oracle}(\widehat{GES},\cdot)$ against $\hat{R}^J_{\bar{\iota},w}(\widehat{GES},\cdot)$ with fitted regression lines. The simulation settings consist of: a sample size of 10, all graph sizes, linear link functions, Normal noise, Do-and-Shift interventions, and different probabilities of an intervention (color-coded). Points on the diagonal indicate a good performance of $\widehat{R}^J_{\bar{\iota},w}(\widehat{GES},\cdot)$ when estimating $\hat{R}^J_{\bar{\iota},oracle}(\widehat{GES},\cdot)$.

### 3.3 PERFORMANCE OF THE DESCENDANT ESTIMATION AND OVERFITTING

Figures 9 to 11 show the performance of the descendant estimation procedure. We plot the naive risk estimator (Equation (5)) under Assumption 1 against the standard naive risk estimator. Points on the diagonal indicate a perfect recovery of the descendants. In each figure the top plot shows the result for the sample size 10 and the bottom plot for the sample size 1000. Figure 9 considers the linear Normal case and shows good results also for the smaller sample size. A larger sample size is needed for the linear log-normal case shown in Figure 10 as suggested in Section 4.2 of the main paper. Finally, Figure 11 shows that for this mis-specified setting good recovery is not possible using t-tests even for a very large sample size (actually, the larger sample size hurts the performance). Figures 9 and 10 show that we did not face any overfitting issues. Otherwise the points should deviate from the diagonal.

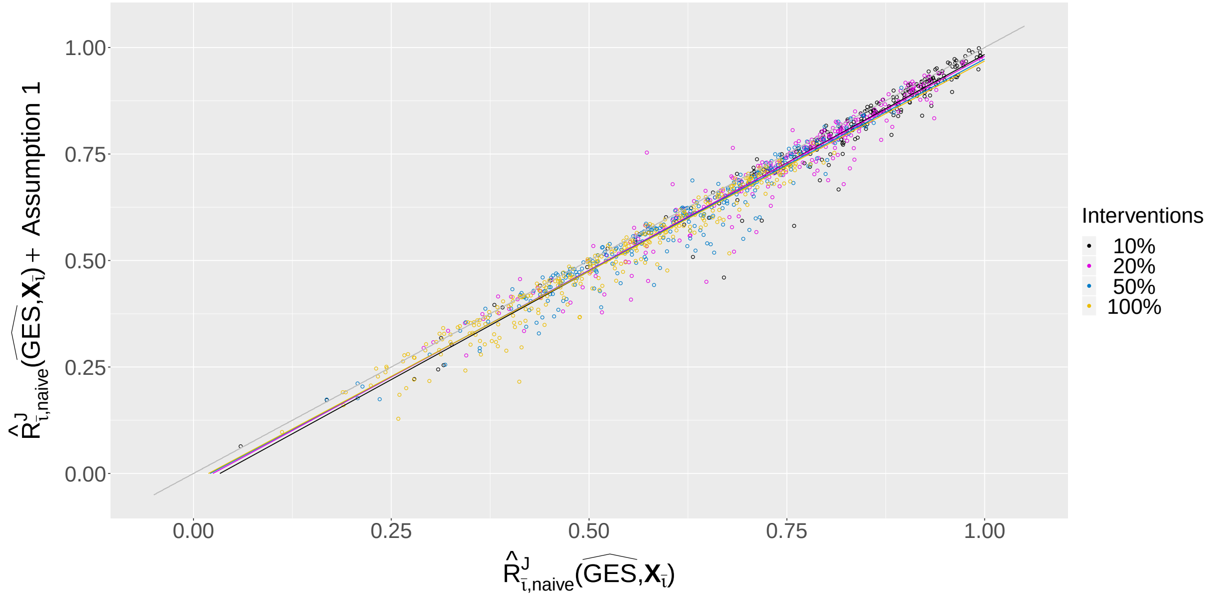


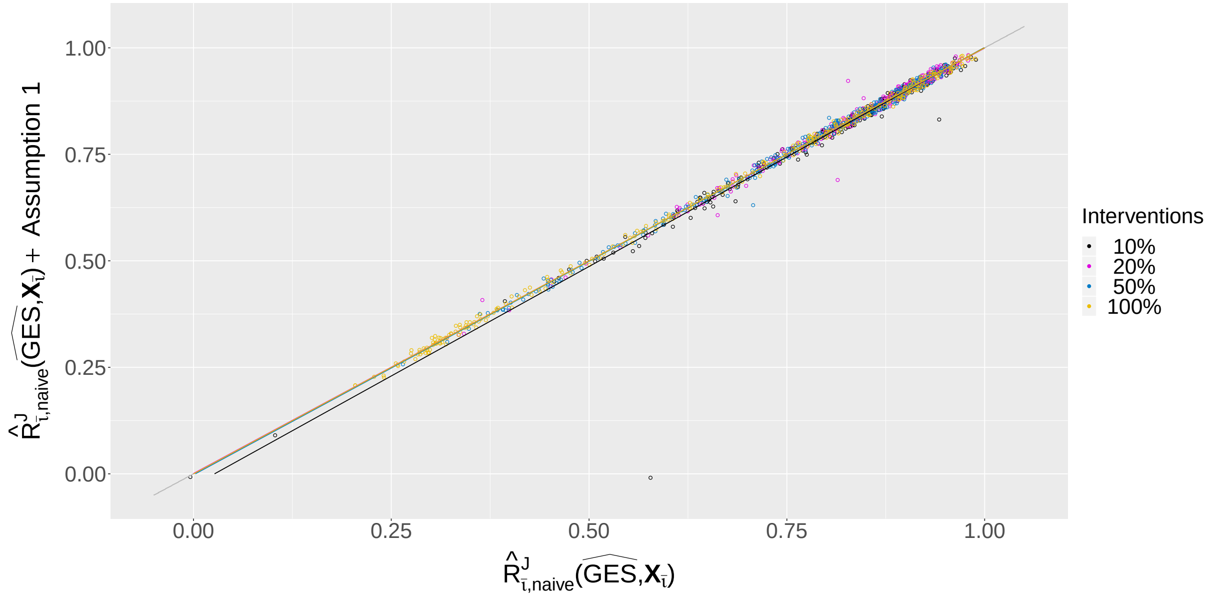


Figure 9: Scatterplots of $\hat{R}^J_{\imath,naive}(\widehat{GES},\cdot)$ under Assumption 1 against $\hat{R}^J_{\imath,naive}(\widehat{GES},\cdot)$ with fitted regression lines. The simulation settings consist of: a sample size of 10 (top) and 1000 (bottom), all graph sizes, linear link functions, Normal noise, Do-and-Shift interventions, and different probabilities of an intervention (color-coded). Points on the diagonal indicate a good performance of the descendants estimation procedure and the lack of overfitting.

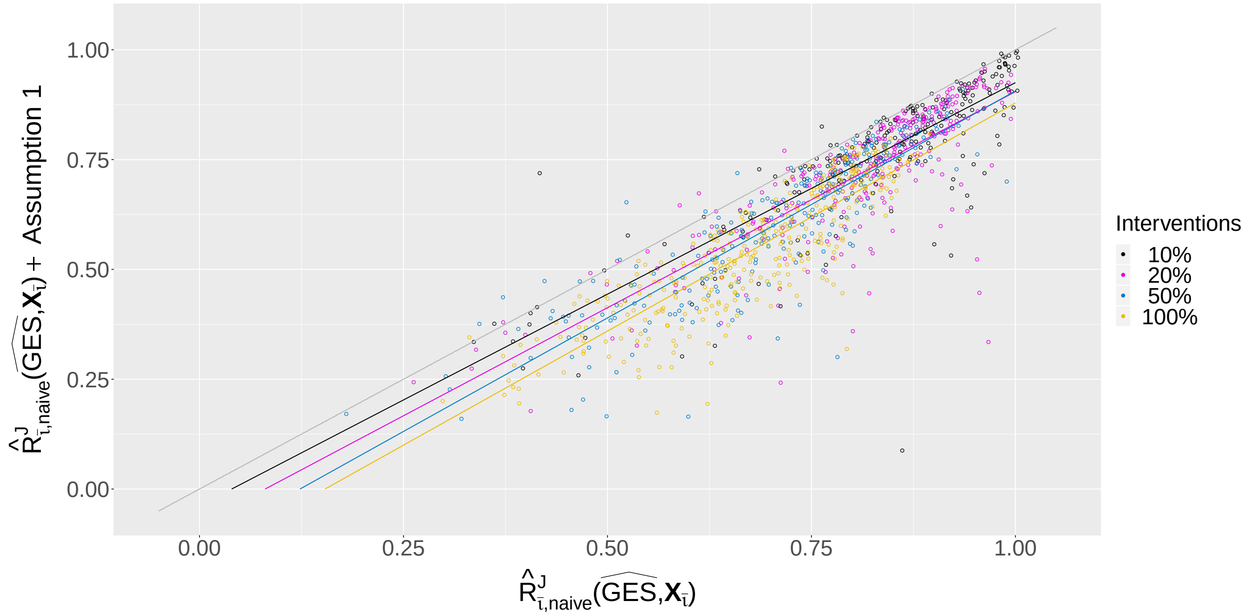


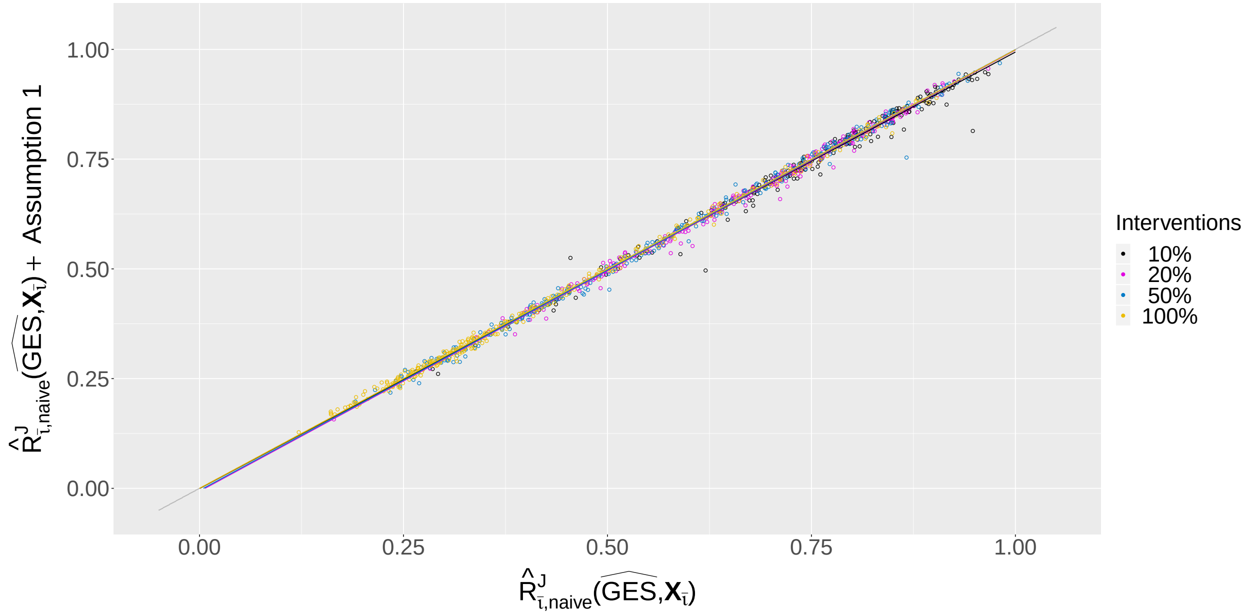


Figure 10: Scatterplots of $\hat{R}^J_{\bar{\iota},naive}(\widehat{GES},\cdot)$ under Assumption 1 against $\hat{R}^J_{\bar{\iota},naive}(\widehat{GES},\cdot)$ with fitted regression lines. The simulation settings consist of: a sample size of 10 (top) and 1000 (bottom), all graph sizes, linear link functions, log-Normal noise, Do-and-Shift interventions, and different probabilities of an intervention (color-coded). Points on the diagonal indicate a good performance of the descendants estimation procedure and the lack of overfitting.

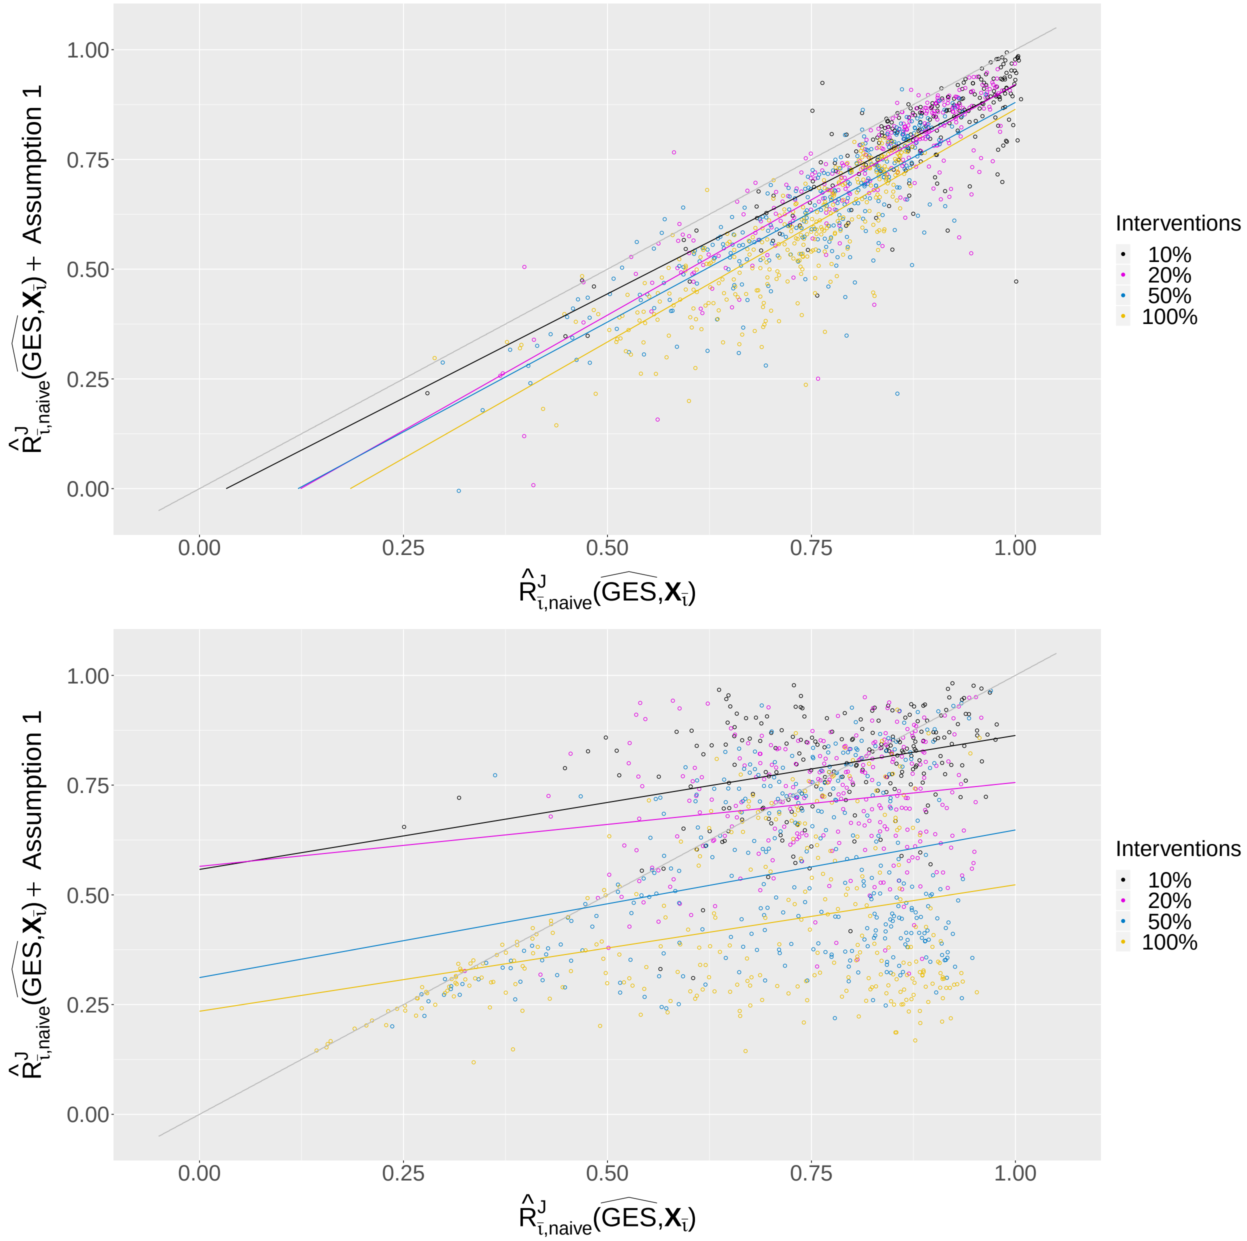


Figure 11: Scatterplots of $\hat{R}^J_{\bar{\iota},naive}(\widehat{GES},\cdot)$ under Assumption 1 against $\hat{R}^J_{\bar{\boldsymbol{\iota}},naive}(\widehat{GES},\cdot)$ with fitted regression lines. The simulation settings consist of: a sample size of 10 (top) and 1000 (bottom), all graph sizes, sigmoidal link functions, log-Normal noise, Do-and-Shift interventions, and different probabilities of an intervention (color-coded). Points on the diagonal indicate a good performance of the descendants estimation procedure and the lack of overfitting.

## References

Heinze-Deml, C., Maathuis, M. H., & Meinshausen, N. (2018). Causal Structure Learning. *Annu. Rev. Stat. Appl.*, *5*, 371-391.
